# Supplementary material for: Jedi: Entropy-based Localization and Removal of Adversarial Patches
Source: arXiv:2304.10029 source file (2023-04-20)
Supplement: Supplementary file 1 [file Appendix.tex]

\noindent\textbf{Parameters exploration}\\
The first parameter considered is the size of the sliding window used for local entropy calculation. The recovery rate and average precision for each window size considered is shown in Figure \ref{fig_4_1}.
%\textcolor{red}{-- maybe we can send this to supplementary materials ?}

\begin{figure}[htp]
  \centering
  \includegraphics[scale = 0.7]{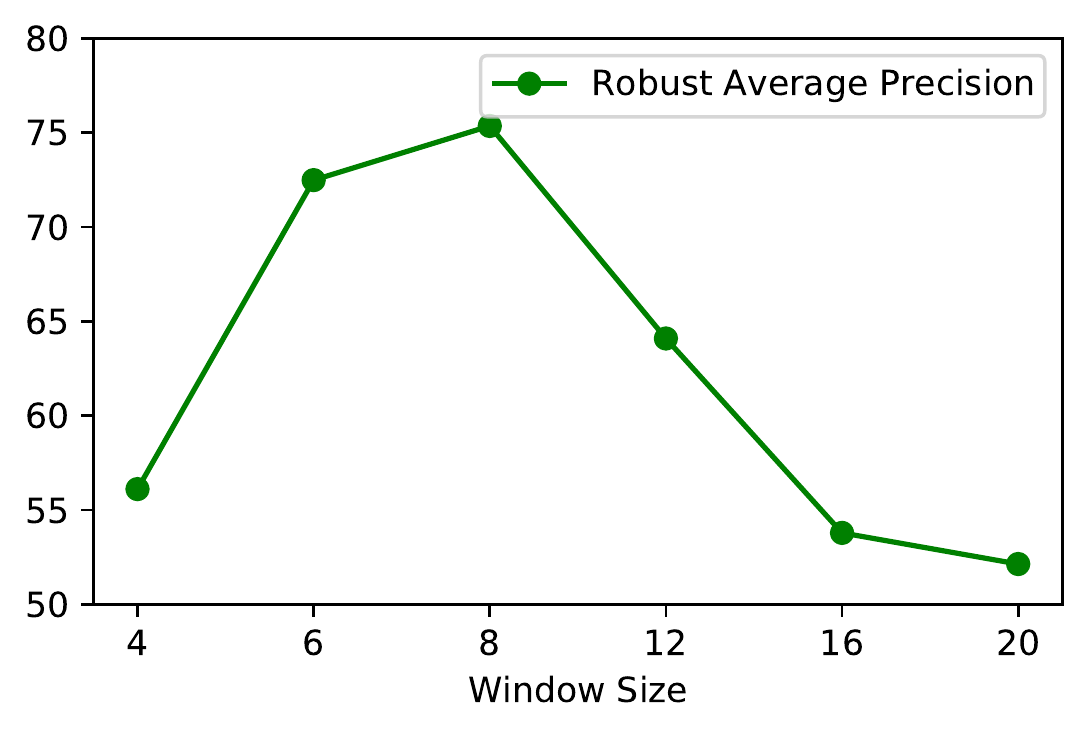}
  \caption{Robust Average Precision for different window sizes}
  % \textcolor{red}{X axis and legend don't match}
  \label{fig_4_1}
\end{figure}

These results show that beyond a certain size, the chosen window generates an imprecise inpainting mask, leading to lower recovery rates. This phenomenon is also observed for very small window sizes, as the entropy of smaller windows is more likely to be below the inpainting threshold. These results show that there is an optimal window size that corresponds to the image's resolution. Therefore, using a static window size is counterproductive; We adopt a dynamic window size equal to $1\%$ of the images largest dimension, with a minimum size of $8$ pixels.

%\smallskip

The second parameter we explore is the stride of the local entropy window. We use the same sample dataset as the previous experiment and a window size of 8 pixels. The results are show in Table \ref{tab:tab3}.

\begin{table}[h!]
    \centering
    \caption{Effect of window stride on defense performance}
    \begin{tabular}{@{}l|lll@{}}
        \toprule
        \textbf{Stride} & \multicolumn{1}{c}{\textbf{1}} & \multicolumn{1}{c}{\textbf{4}} & \multicolumn{1}{c}{\textbf{8}} \\ \midrule
        Clean               & 100\%   & 100\%   & 100\%   \\
        Patch Success Rate  & 72.20\% & 72.20\% & 72.20\% \\
        Detected Patches    & 92,20\% & 90.50\% & 87.45\% \\
        Robust Avg Precision& 81.50\% & 79.73\% & 75.35\% \\ \bottomrule
        \end{tabular}
    \label{tab:tab3}
\end{table}

%\ihsen{please revise this with the corresponding table $\rightarrow$} 
The results show that lowering the window stride leads to a better performing defense, as a more granular local entropy calculation results in a more accurate inpainting mask. However, beyond a certain point, the improvements brought by lowering the window stride are quickly outpaced by the negative effect of exponentially increasing the number of entropy calculations. Therefore, we set the window stride to be equal to half of the window size as this value keeps most of the performance gains from lowering the window stride while keeping calculation time reasonable.

\textbf{Alternate method for creating the patch mask}

An earlier version of our work investigated an alternate method of creating 
we have evaluated an alternative method for creating the mask that locates the adversarial patch. This method follows the same framework as our main proposed approach, but the methods for determining the high entropy kernels and obtaining the full shape of the patch differ:

First, to determine the locations of high entropy kernels, a local entropy heatmap is established using a sliding window, and the kernels are located by keeping only the peaks of this heatmap: Only windows whose entropy value exceeds the top-k\% of the maximum entropy value are considered as high entropy kernels, the rest of the heatmap is discarded.

Next, instead of using an autoencoder to determine the final mask, we "expand" our kernels to fit the shape of the adversarial patch: We compare each high entropy kernel with the windows that surround it, in an $n$-window radius using a similarity metric. If the neighboring window is similar to the high entropy kernel, it is added to the final patch mask.

The similarity metric we use in this method is mutual information. For each kernel, we determine the self-mutual information of the kernel as a baseline, and we compare the mutual information between the high entropy kernel and candidate window for expansion. If the ratio of this mutual information value relative to the self-mutual information is higher than the threshold. The candidate window is considered as part of the adversarial patch.

These two steps produce a mask that shows the location of the adversarial patch, we then filter this mask and use it to apply the inpainting method in the same way as discussed in textbfs B and C of Section \ref{sec:prop} that presents our main proposed approach. 

The performance of this alternative approach and the difference in recovery rates when compared against our main method are show in table \ref{tab:annex_alt}: 

\begin{table}
\caption{Performance of the alternative patch localization method with comparison to the main method}
\label{tab:annex_alt}
\begin{tabular}{@{}l|llll@{}}
\toprule
Experiment                                                                                         & Metric            & Main    & Alternative \\ \midrule
\multirow{2}{*}{\begin{tabular}[c]{@{}l@{}}ImageNet\\ + \cite{lavan}\\ + InceptionV3\end{tabular}}        & Robust Accuracy          & 55.26\% & 51.36\%    \\ \\
                                                                                                   & Recovery Rate \    & 75.26\% & 70.45\%     \\ \midrule
\multirow{2}{*}{\begin{tabular}[c]{@{}l@{}}Pascal VOC 07\\ + \cite{advpatch}\\ + ResNet50\end{tabular}} & Robust Accuracy          & 66.40\% & 66.60\%   \\ \\
                                                                                                   & Recovery Rate     & 82.74\% & 83.51\%    \\ \midrule
\multirow{2}{*}{\begin{tabular}[c]{@{}l@{}}CASIA\\ + \cite{yolopatch}\\ + YOLOv2\end{tabular}}           & Robust Avg & 88.21\% & 70.52\%   \\ & Precision & & &  \\
                                                                                                   & Recovery Rate     & 94.38\% & 84.15\%   \\ \bottomrule
\end{tabular}
\end{table}

This method's results are inferior in most cases to our main method's results, and equal in the best of cases. Furthermore, this approach may have some scalability issues, especially in images with higher resolutions and when using smaller window sizes or when there is a large number of high entropy kernels in the image. Nonetheless, this alternative approach may have its merits in situations where it is impractical to use an autoencoder or if preparing the clean dataset entropy distribution is not possible.

\textbf{Full result tables}

In this subsection of the supplementary materials, we include the full tables with detailed results of each CNN and adversarial patch we have applied to the four datasets used in our evaluation:

\begin{itemize}
    \item ImageNet results are shown in table \ref{tab:full_res_imagenet}
    \item Pascal VOC 07 results are shown in table \ref{tab:full_res_pascal}
    \item CASIA results are shown in table \ref{tab:full_res_casia}
    \item INRIA results are shown in table \ref{tab:full_res_inria}
\end{itemize}

\begin{table*}[]
\centering
\caption{Evaluation results for the experiments performed on ImageNet}
\label{tab:full_res_imagenet}
\begin{tabular}{@{}lllllll@{}}
\toprule
\multicolumn{7}{l}{\textbf{Patch: \cite{advpatch}, trained on Imagenet}}                                                                     \\ \midrule
\multicolumn{1}{l|}{Classifier}           & VGG-16  & VGG-19  & ResNet-18 & ResNet-50 & ResNet-101 & InceptionV3 \\ \midrule
\multicolumn{1}{l|}{Clean Accuracy}       & 68.80\% & 69.87\% & 66.56\%   & 74.10\%   & 75.53\%    & 67.65\%     \\
\multicolumn{1}{l|}{Patch Success Rate}   & 31.16\% & 31.96\% & 29.34\%   & 49.02\%   & 31.05\%    & 23.10\%     \\
\multicolumn{1}{l|}{Adversarial Accuracy} & 50.04\% & 50.37\% & 50.45\%   & 39.26\%   & 54.45\%    & 54.93\%     \\ \midrule
\multicolumn{1}{l|}{Patch Detection Rate} & 85.31\% & 85.31\% & 85.31\%   & 85.31\%   & 85.31\%    & 85.31\%     \\
\multicolumn{1}{l|}{Robust Accuracy}      & 57.86\% & 58.53\% & 58.20\%   & 64.34\%   & 66.28\%    & 59.09\%     \\
\multicolumn{1}{l|}{Recovery Rate}        & 45.18\% & 44.75\% & 49.87\%   & 66.95\%   & 55.22\%    & 43.72\%     \\
\multicolumn{1}{l|}{Lost Predictions}     & 5.38\%  & 4.88\%  & 5.15\%    & 2.77\%    & 3.48\%     & 5.98\%      \\ \midrule
\multicolumn{7}{l}{\textbf{Patch: \cite{lavan}, trained on Imagenet}}                                                                        \\ \midrule
\multicolumn{1}{l|}{Classifier}           & VGG-16  & VGG-19  & ResNet-18 & ResNet-50 & ResNet-101 & InceptionV3 \\ \midrule
\multicolumn{1}{l|}{Clean Accuracy}             & 68.80\% & 69.87\% & 66.56\%   & 74.10\%   & 75.53\%    & 67.65\%     \\
\multicolumn{1}{l|}{Patch Success Rate}   & 25.86\% & 29.33\% & 28.00\%   & 19.57\%   & 20.52\%    & 93.22\%     \\
\multicolumn{1}{l|}{Adversarial Accuracy}       & 54.30\% & 52.43\% & 51.31\%   & 62.61\%   & 62.76\%    & 4.82\%      \\ \midrule
\multicolumn{1}{l|}{Patch Detection Rate} & 89.22\% & 89.22\% & 89.22\%   & 89.22\%   & 89.22\%    & 89.22\%     \\
\multicolumn{1}{l|}{Robust Accuracy}            & 58.73\% & 58.50\% & 58.37\%   & 65.72\%   & 66.68\%    & 55.26\%     \\
\multicolumn{1}{l|}{Recovery Rate}        & 38.54\% & 41.29\% & 46.65\%   & 36.03\%   & 39.47\%    & 75.26\%     \\
\multicolumn{1}{l|}{Lost Predictions}     & 5.10\%  & 6.09\%  & 3.78\%    & 4.28\%    & 4.63\%     & 3.33\%      \\ \bottomrule
\end{tabular}
\end{table*}

\begin{table*}[]
\centering
\caption{Evaluation results for the experiments performed on Pascal VOC 07}
\label{tab:full_res_pascal}
\begin{tabular}{@{}lllllll@{}}
\toprule
\multicolumn{7}{l}{\textbf{Patch: \cite{advpatch}, trained on Imagenet}}                                                           \\ \midrule
\multicolumn{1}{l|}{Classifier}           & VGG-16  & VGG-19  & ResNet-18 & ResNet-50 & ResNet-101 & InceptionV3 \\ \midrule
\multicolumn{1}{l|}{Clean Accuracy}       & 77.36\% & 77.12\% & 70.78\%   & 72.17\%   & 74.09\%    & 70.17\%     \\
\multicolumn{1}{l|}{Patch Success Rate}   & 16.86\% & 11.99\% & 17.95\%   & 18.63\%   & 18.29\%    & 19.25\%     \\
\multicolumn{1}{l|}{Adversarial Accuracy} & 66.98\% & 70.78\% & 61.41\%   & 61.65\%   & 63.61\%    & 59.77\%     \\ \midrule
\multicolumn{1}{l|}{Patch Detection Rate} & 89.51\% & 89.51\% & 89.51\%   & 89.51\%   & 89.51\%    & 89.51\%     \\
\multicolumn{1}{l|}{Robust Accuracy}      & 71.53\% & 72.27\% & 67.33\%   & 67.73\%   & 70.30\%    & 64.82\%     \\
\multicolumn{1}{l|}{Recovery Rate}        & 53.10\% & 38.21\% & 58.51\%   & 59.31\%   & 64.68\%    & 60.39\%     \\
\multicolumn{1}{l|}{Lost Predictions}     & 3.39\%  & 2.23\%  & 2.54\%    & 2.54\%    & 2.77\%     & 4.63\%      \\ \midrule
\multicolumn{7}{l}{\textbf{Patch: \cite{lavan}, trained on Imagenet}}                                                                        \\ \midrule
\multicolumn{1}{l|}{Classifier}           & VGG-16  & VGG-19  & ResNet-18 & ResNet-50 & ResNet-101 & InceptionV3 \\ \midrule
\multicolumn{1}{l|}{Clean Accuracy}       & 77.36\% & 77.12\% & 70.78\%   & 72.17\%   & 74.09\%    & 70.17\%     \\
\multicolumn{1}{l|}{Patch Success Rate}   & 10.34\% & 9.03\%  & 13.10\%   & 13.63\%   & 15.32\%    & 23.08\%     \\
\multicolumn{1}{l|}{Adversarial Accuracy} & 71.79\% & 72.80\% & 65.21\%   & 65.43\%   & 65.67\%    & 56.89\%     \\ \midrule
\multicolumn{1}{l|}{Patch Detection Rate} & 91.33\% & 91.33\% & 91.33\%   & 91.33\%   & 91.33\%    & 91.33\%     \\
\multicolumn{1}{l|}{Robust Accuracy}      & 72.37\% & 72.94\% & 66.96\%   & 67.43\%   & 70.23\%    & 64.36\%     \\
\multicolumn{1}{l|}{Recovery Rate}        & 28.79\% & 24.06\% & 43.79\%   & 44.76\%   & 60.68\%    & 58.23\%     \\
\multicolumn{1}{l|}{Lost Predictions}     & 2.68\%  & 2.62\%  & 2.99\%    & 2.79\%    & 3.51\%     & 3.82\%      \\ \midrule
\multicolumn{7}{l}{\textbf{Patch: \cite{advpatch}, trained on Pascal VOC 07}}                                                              \\ \midrule
\multicolumn{1}{l|}{Classifier}           & VGG-16  & VGG-19  & ResNet-18 & ResNet-50 & ResNet-101 & InceptionV3 \\ \midrule
\multicolumn{1}{l|}{Clean Accuracy}       & 77.36\% & 77.12\% & 70.78\%   & 72.17\%   & 74.09\%    & 70.17\%     \\
\multicolumn{1}{l|}{Patch Success Rate}   & 22.81\% & 20.84\% & 35.35\%   & 63.88\%   & 26.55\%    & 22.42\%     \\
\multicolumn{1}{l|}{Adversarial Accuracy} & 62.32\% & 63.67\% & 48.30\%   & 26.94\%   & 56.91\%    & 57.65\%     \\ \midrule
\multicolumn{1}{l|}{Patch Detection Rate} & 92.62\% & 92.62\% & 92.62\%   & 92.62\%   & 92.62\%    & 92.62\%     \\
\multicolumn{1}{l|}{Robust Accuracy}      & 72.29\% & 72.15\% & 67.14\%   & 66.40\%   & 69.97\%    & 65.53\%     \\
\multicolumn{1}{l|}{Recovery Rate}        & 65.90\% & 60.68\% & 76.43\%   & 82.74\%   & 70.64\%    & 62.77\%     \\
\multicolumn{1}{l|}{Lost Predictions}     & 2.94\%  & 2.38\%  & 2.25\%    & 1.32\%    & 2.41\%     & 3.71\%      \\ \bottomrule
\end{tabular}
\end{table*}

\begin{table*}[]
\centering
\caption{Evaluation results for the experiments performed on CASIA}
\label{tab:full_res_casia}
\begin{tabular}{@{}llll@{}}
\toprule
\multicolumn{4}{l}{\textbf{Patch: \cite{yolopatch}, trained on Wildtrack}}                                    \\ \midrule
\multicolumn{1}{l|}{Detector}                      & YoloV2  & YoloV3  & YoloV4  \\ \midrule
\multicolumn{1}{l|}{Clean Average Precision}       & 91,47\% & 92.47\% & 87.85\% \\
\multicolumn{1}{l|}{Patch Success Rate}            & 26.10\% & 60.55\% & 18.18\% \\
\multicolumn{1}{l|}{Adversarial Average Precision} & 39.60\% & 20.31\% & 58.46\% \\ \midrule
\multicolumn{1}{l|}{Patch Detection Rate}          & 95.31\% & 95.31\% & 95.31\% \\
\multicolumn{1}{l|}{Robust Average Precision}      & 88.21\% & 76.17\% & 85.10\% \\
\multicolumn{1}{l|}{Recovery Rate}                 & 94.38\% & 79.98\% & 89.47\% \\
\multicolumn{1}{l|}{Lost Predictions}              & 0.07\%  & 4.36\%  & 0.26\%  \\ \midrule
\multicolumn{4}{l}{\textbf{Patch: \cite{naturalistic}, trained on CASIA}}                           \\ \midrule
\multicolumn{1}{l|}{Detector}                      & YoloV2  & YoloV3  & YoloV4  \\ \midrule
\multicolumn{1}{l|}{Clean Average Precision}       & 91,47\% & 92.47\% & 87.85\% \\
\multicolumn{1}{l|}{Patch Success Rate}            & 7.09\%  & 63.61\% & 19.72\% \\
\multicolumn{1}{l|}{Adversarial Average Precision} & 76.56\% & 23.53\% & 60.61\% \\ \midrule
\multicolumn{1}{l|}{Patch Detection Rate}          & 95.59\% & 95.59\% & 95.59\% \\
\multicolumn{1}{l|}{Robust Average Precision}      & 85.22\% & 72.68\% & 83.45\% \\
\multicolumn{1}{l|}{Recovery Rate}                 & 82.83\% & 76.95\% & 83.70\% \\
\multicolumn{1}{l|}{Lost Predictions}              & 0.48\%  & 5.03\%  & 0.50\%  \\ \bottomrule
\end{tabular}
\end{table*}

\begin{table*}[]
\centering
\caption{Evaluation results for the experiments performed on INRIA}
\label{tab:full_res_inria}
\begin{tabular}{@{}llll@{}}
\toprule
\multicolumn{4}{l}{\textbf{Patch: \cite{yolopatch}, trained on Wildtrack}}                                    \\ \midrule
\multicolumn{1}{l|}{Detector}                      & YoloV2  & YoloV3  & YoloV4  \\ \midrule
\multicolumn{1}{l|}{Clean Average Precision}       & 51.11\% & 81.51\% & 85.77\% \\
\multicolumn{1}{l|}{Patch Success Rate}            & 61.15\% & 33.88\% & 37.02\% \\
\multicolumn{1}{l|}{Adversarial Average Precision} & 12.17\% & 41.80\% & 38.44\% \\ \midrule
\multicolumn{1}{l|}{Patch Detection Rate}          & 38.80\% & 38.80\% & 38.80\% \\
\multicolumn{1}{l|}{Robust Average Precision}      & 28.03\% & 53.07\% & 50.71\% \\
\multicolumn{1}{l|}{Recovery Rate}                 & 41.88\% & 43.61\% & 32.57\% \\
\multicolumn{1}{l|}{Lost Predictions}              & 1.14\%  & 3.39\%  & 2.03\%  \\ \midrule
\multicolumn{4}{l}{\textbf{Patch: \cite{naturalistic}, trained on INRIA}}                           \\ \midrule
\multicolumn{1}{l|}{Detector}                      & YoloV2  & YoloV3  & YoloV4  \\ \midrule
\multicolumn{1}{l|}{Clean Average Precision}       & 51.11\% & 81.51\% & 85.77\% \\
\multicolumn{1}{l|}{Patch Success Rate}            & 34.22\% & 29.40\% & 28.94\% \\
\multicolumn{1}{l|}{Adversarial Average Precision} & 33.04\% & 52.22\% & 48.71\% \\ \midrule
\multicolumn{1}{l|}{Patch Detection Rate}          & 56.56\% & 56.56\% & 56.56\% \\
\multicolumn{1}{l|}{Robust Average Precision}      & 47.04\% & 65.11\% & 65.49\% \\
\multicolumn{1}{l|}{Recovery Rate}                 & 68.39\% & 51.27\% & 53.92\% \\
\multicolumn{1}{l|}{Lost Predictions}              & 2.35\%  & 2.33\%  & 2.40\%  \\ \bottomrule
\end{tabular}
\end{table*}

\section{Illustration of entropy budget on the generated patches}
\begin{figure}[H]
     \centering
     \begin{subfigure}[b]{0.15\textwidth}
         \centering
         \includegraphics[width=0.7\textwidth]{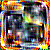}
         \caption{No entropy limit}
         \label{fig:y equals x}
     \end{subfigure}
     \hfill
     \begin{subfigure}[b]{0.15\textwidth}
         \centering
         \includegraphics[width=0.7\textwidth]{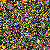}
         \caption{Entropy = 7}
         \label{fig:three sin x}
     \end{subfigure}
     \hfill
     \begin{subfigure}[b]{0.15\textwidth}
         \centering
         \includegraphics[width=0.7\textwidth]{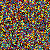}
         \caption{Entropy = 5}
         \label{fig:five over x}
     \end{subfigure}
        \caption{Samples of the adaptive patch under entropy limits}
        \label{fig_adapt_entr}
\end{figure}

\section{Low Entropy Adaptive Patch Generation Algorithm}

\begin{algorithm}
    \caption{Low entropy patch generation algorithm}
    \label{alg1}
    \begin{algorithmic}[1]
        \State \textbf{Input:}{ $n_{epochs}$: number of training epochs ,$I_{train}$ Training image set,$params$: Patch generation parameters, $checkFreq$: Frequency of entropy checks , $\varepsilon$: entropy limit}
        \State \textbf{Output:}{ Low entropy adversarial patch}
        \For {$e \in [1,n_{epochs}]$}
            \For {$im \in I_{train}$}
                \State patch = \textit{PatchTraining}(params)
                \If{$it \% checkFreq == 0$ }
                \State \textit{/*Repeat each \textit{checkFreq} iterations*/}
                    \State patchEntropy $\xleftarrow{}$ \textit{Entropy}(patch)
                    \While{$patchEntropy > \varepsilon$} 
                        \State colorList $\xleftarrow{}$ \textit{random}(0,255,10)
                        \State patch $\xleftarrow{}$ reduceEntropy(patch,colorList)
                    \EndWhile
                    \State $patchEntropy$ $\xleftarrow{}$ \textit{entropy}(patch)
                \EndIf
            \EndFor
        \EndFor
        \State
        \State \textbf{function} \textit{reduceEntropy}(patch,colorList)
        \State \textit{/*Find best patch among random color removal tries*/}
        \For{$c \in colorList$}
        \State nearestColor $\xleftarrow{}$ \textit{findNearestColor}(c)
        \State newPatch[c] $\xleftarrow{}$ \textit{replaceColor}(patch, c, nearestColor)
        \State newPatchASR[c] $\xleftarrow{}$ \textit{testSuccessRate}(newPatch[c])
        \EndFor
        \State bestPatch $\xleftarrow{}$ \textit{argmax}(newPatchASR)
        \State \textbf{return} bestPatch
        \State \textbf{end function}
    \end{algorithmic}
\end{algorithm}
